# Supplementary material for: 6DOPE-GS: Online 6D Object Pose Estimation using Gaussian Splatting
Source: arXiv:2412.01543 source file (2025-04-03)
Supplement: Supplementary file 1 [file 06_appendix.tex]

% \section{Appendix Section}
% \label{sec:appendix_section}
% To split the supplementary pages from the main paper, you can use \href{https://support.apple.com/en-ca/guide/preview/prvw11793/mac#:~:text=Delete%20a%20page%20from%20a,or%20choose%20Edit%20%3E%20Delete).}{Preview (on macOS)}, \href{https://www.adobe.com/acrobat/how-to/delete-pages-from-pdf.html#:~:text=Choose%20%E2%80%9CTools%E2%80%9D%20%3E%20%E2%80%9COrganize,or%20pages%20from%20the%20file.}{Adobe Acrobat} (on all OSs), as well as \href{https://superuser.com/questions/517986/is-it-possible-to-delete-some-pages-of-a-pdf-document}{command line tools}.
\clearpage
\setcounter{page}{1}
\maketitlesupplementary

% \textbf{See BundleSDF, FoundationPose and Gen6D supplementary for inspiration}\\

\section{Joint Optimization of 2D Gaussians and Keyframe Poses}% via Structural Photometric Self-Supervision} 
% \section{Calculation of Keyframe Pose Gradients}
% \label{sec:kf-gradients}
% \begin{itemize}
%     \item 2D Gaussian Splatting Differentiable Rasterization
%     \item Projecting to Canonical Coordinates
%     \item Pose Gradients with respect to losses (with learnable transformation)
% \end{itemize}

% We use the automatic differentiation in PyTorch~\cite{paszke2017automatic} 
Once we obtain an initial set of coarse keyframe poses, we jointly optimize the 2D Gaussians and the keyframe poses based on the photometric and structural losses used in in~\cite{huang2DGaussianSplatting2024}. These losses include a color consistency loss $\mathcal{L}_c$, a depth consistency loss $\mathcal{L}_d$, a depth distortion loss $\mathcal{L}_{dd}$, and a normal alignment loss $\mathcal{L}_n$. The losses are computed between the rendered and observed images within the pixels covered in the object segmentation mask \(\mathcal{M}\). To further reduce camera depth noise, we additionally use the Huber loss.

% The color consistency loss $\mathcal{L}_c$ is the $L_1$ loss between the observed and the rendered images calculated as
% \begin{equation}
%     \mathcal{L}_c = \frac{1}{|\mathcal{M}|}\sum_{\boldsymbol{p}\in\mathcal{M}}|\hat{c}(\boldsymbol{p}) - c(\boldsymbol{p})|
% \end{equation}
% where $c(\boldsymbol{p})$ is the observed pixel color and $\hat{c}(\boldsymbol{p}) = = \sum_{i \in N} \omega_ic_i$ is the rendered color at a pixel $\boldsymbol{p}$. 

The color consistency loss $\mathcal{L}_c$ and the depth consistency loss $\mathcal{L}_d$ is the $L_1$ loss between the observed and the rendered images. The losses are calculated after projecting the Gaussians onto the image frame. Specifically, the Gaussians are ordered according to their ascending z-depth in the camera frame after which the contribution of each Gaussian to the loss is weighted based on their opacity and Gaussian density. This process is called $\alpha$-blending. We represent the blending weight of each of the $N$ ordered Gaussians as

\begin{equation}
    \omega_i(\boldsymbol{p}) = \alpha_i G^{2D}_i(\boldsymbol{p}) \prod_{j=1}^{i-1} (1 - \alpha_jG^{2D}_j(\boldsymbol{p})) \hspace{1em};\hspace{1em} \forall i\in N
\end{equation}

We then calculate the color consistency loss $\mathcal{L}_c$ and the depth consistency loss $\mathcal{L}_d$ as

\begin{equation}
    \mathcal{L}_c = \frac{1}{|\mathcal{M}|}\sum_{\boldsymbol{p}\in\mathcal{M}}|\hat{c}(\boldsymbol{p}) - c(\boldsymbol{p})|
\end{equation}
\begin{equation}
    \mathcal{L}_d = \frac{1}{|\mathcal{M}|}\sum_{\boldsymbol{p}\in\mathcal{M}}\rho(|\hat{d}(\boldsymbol{p}) - d(\boldsymbol{p})|)
\end{equation}
where $\rho(\cdot)$ is the Huber loss, $c(\boldsymbol{p})$ and $d(\boldsymbol{p})$ are the observed color and depth, and $\hat{c}(\boldsymbol{p})~=~\sum_{i\in N}c_i\omega_i(\boldsymbol{p})$ and $\hat{d}(\boldsymbol{p})~=~\sum_{i\in N}d_i\omega_i(\boldsymbol{p})$ are the rendered color and depth at a pixel $\boldsymbol{p}$.

% When replacing the Gaussian's color in Eq.~\ref{eq:gs-forward-rendering} with the z-depth, we can similarly render the depth of a pixel $\boldsymbol{p}$ as 
% \begin{equation}
% \label{eq:gs-forward-depth-rendering}
% \hat{d}(\boldsymbol{p}) = \sum_{i \in N} z_i \alpha_i G^{2D}_i(\boldsymbol{p}) \prod_{j=1}^{i-1} (1 - \alpha_jG^{2D}_j(\boldsymbol{p}))
% \end{equation}

The depth distortion loss clusters the 2D Gaussians along the ray path, minimizing gaps between intersected Gaussians and enhancing depth accuracy. 
\begin{equation}
\mathcal{L}_{dd} = \sum_{i,j \in N} \omega_i \omega_j |z_i - z_j|
\end{equation}
where $\omega_i$ is the blending weight for the $i^{th}$ Gaussian intersection, and \( z_i \) denotes the depth of each intersection point. Adjusting the intersection depth \( z_i \) to encourage the concentration of splats along the ray. 

% The normal loss $\mathcal{L}_{\text{n}}$ further refines object shape by aligning each Gaussian’s normal with the local surface gradient.
% \begin{equation}
% \mathcal{L}_n = \sum_{i\in N} \omega_i \left( 1 - \boldsymbol{\hat{n}}_i^{\top} \boldsymbol{n}_i \right)
% \end{equation}
% where $\boldsymbol{\hat{n}}_i$ represents the normal of the 2D Gaussian's surface oriented toward the camera, and $\boldsymbol{n}_i$ is the normal estimated by the depth gradient.
The normal loss $\mathcal{L}_{\text{n}}$ further refines object shape by aligning each Gaussian’s normal with the local surface gradient.
\begin{equation}
\mathcal{L}_n = \sum_{\boldsymbol{p}\in\mathcal{M}} 1 - \boldsymbol{\hat{n}}(\boldsymbol{p})^{\top} \boldsymbol{n}(\boldsymbol{p})
\end{equation}
where $\boldsymbol{\hat{n}}(\boldsymbol{p})$ and $\boldsymbol{n}(\boldsymbol{p})$ are the normals at pixel $\boldsymbol{p}$ estimated by the gradient of the rendered and observed depth images respectively. By aligning the splat normal with the estimated normal, we ensure that the 2D splats accurately approximate the local object surface.

For refining the keyframe poses, a learnable affine transformation $\boldsymbol{T}_k\in SE(3)$ of the k$^{th}$  keyframe is applied to the 2D Gaussians similar to~\cite{matsukiGaussianSplattingSLAM2024, yugayGaussianSLAMPhotorealisticDense2024}. The transformation $\boldsymbol{T}_k$ is represented by a rotation $\boldsymbol{R}_k \in SO(3)$ and a translation $t_k \in \mathbb{R}^3$. We learn the transformations along with the Gaussians by minimizing the above-mentioned losses obtained by projecting each Gaussian $G_i\in\mathcal{G}$ onto each selected keyframe pose $\boldsymbol{T}_k\in\mathcal{K}$ as
\begin{equation}
\begin{aligned}
\mathcal{G}^*, \mathcal{K}^* = \arg\min_{\mathcal{G},\mathcal{K}}\sum_{k\in|\mathcal{K}|}&\lambda_c\mathcal{L}_c(\hat{I}(\boldsymbol{T}_k \odot \mathcal{G}), I_{k}) \\
+&\lambda_d\mathcal{L}_d(\hat{D}(\boldsymbol{T}_k \odot \mathcal{G}), D_{k})\\
+&\lambda_{dd}\mathcal{L}_{dd} + \lambda_n\mathcal{L}_n
% +&\lambda_n\mathcal{L}_n(\hat{D}(\boldsymbol{T}_k \odot \mathcal{G}), D_{k})
\end{aligned}
\end{equation}
where $\hat{I}$ and $\hat{D}$ are the rendered color and depth images obtained by projecting the Gaussians $\mathcal{G}$ to the $k^{th}$ keyframe pose $\boldsymbol{T}_k$ and $I_k$, $D_k$ represent the observed color and depth images of the $k^{th}$ keyframe. $\lambda_c$, $\lambda_d$, $\lambda_{dd}$ and $\lambda_n$ are the relative weights for the color, depth, depth distortion and normal losses respectively.

\section{Metrics}
To evaluate 6-DoF object pose estimation, we calculate the Area Under Curve (AUC) percentage based on the ADD and ADD-S metrics. The ADD metric determines the average Euclidean distance between corresponding points on the 3D object model after transformation by the predicted and ground truth poses.
\begin{equation}
    \text{ADD} = \frac{1}{N} \sum_{i=1}^N \| (R x_i + t) - (R_{\text{gt}} x_i + t_{\text{gt}}) \|,
\end{equation}
where \(N\) represents the number of points in the 3D object model, \(x_i\) denotes a point on the model, \(R\) and \(t\) are the predicted rotation matrix and translation vector, and \(R_{\text{gt}}\) and \(t_{\text{gt}}\) are their ground truth counterparts. A lower ADD value indicates a more accurate pose estimation. The estimation is considered successful if the ADD is within a specific threshold. For symmetric objects, where distinct poses may appear identical (e.g., a cylindrical object rotated by 180°), the ADD-S metric is more appropriate. Instead of directly pairing corresponding points, ADD-S measures the average distance between a transformed model point and its nearest neighbor in the ground truth-transformed model.
\begin{equation}
    \text{ADD-S} = \frac{1}{N} \sum_{i=1}^N \min_{x_j \in \mathcal{M}} \| (R x_i + t) - (R_{\text{gt}} x_j + t_{\text{gt}}) \|,
\end{equation}
where \(x_j \in \mathcal{M}\) denotes the set of all 3D points on the object model. This formulation accounts for the ambiguities inherent to symmetric objects, providing a more robust evaluation of pose estimation.

We assess 3D shape reconstruction performance by calculating the chamfer distance between the reconstructed and ground-truth points, adopting the symmetric formulation.
\begin{equation}
\text{CD}(P, Q) = \frac{1}{|P|} \sum_{p \in P} \min_{q \in Q} \| p - q \|^2 + \frac{1}{|Q|} \sum_{q \in Q} \min_{p \in P} \| q - p \|^2
\end{equation}
To extract meshes from reconstructed 2D splats, we render depth maps of the training views by projecting the depth values of the splats onto the pixels. Truncated Signed Distance Fusion (TSDF) is then used to fuse the reconstructed depth maps, implemented using Open3D~\cite{zhou2018open3d}. During TSDF fusion, we set the voxel size to 0.002 and the truncation threshold to 0.02. Additionally, we extend BundleSDF to render depth maps and apply the same surface reconstruction technique to ensure a fair comparison.

\section{Implementation Details}
For the object masks in the YCBInEOAT dataset, we utilize the original masks provided in the dataset. For the HO3D dataset, we use the masks extracted XMem~\cite{chengXMemLongTermVideo2022}, as done in BundleSDF~\cite{wenBundleSDFNeural6DoF2023}. In real-time scenarios, we manually input the initial object location as a prompt for a random frame from the camera. Based on the prompted image, SAM2~\cite{raviSAM2Segment} segments the target object across video frames in real-time. 

During coarse pose estimation, a new frame is designated as a keyframe if it has more than 10 feature correspondences with the frames in memory. For online graph optimization, we retain the configuration of BundleSDF~\cite{wenBundleSDFNeural6DoF2023}, restricting the number of frames involved in pose graph optimization to a maximum of 10.

For the Gaussian object field, we transform all graph-optimized camera poses into the OpenGL camera representation, which is utilized for Gaussian splatting. OpenGL adopts a right-handed coordinate system with the camera facing the negative z-axis, whereas OpenCV uses a right-handed system with the camera facing the positive z-axis. Using the information from the first frame, we estimate the object size and rescale and translate all camera poses and point clouds to ensure the generated Gaussians fit within a canonical space ranging from -1 to 1. Starting from the 10th keyframe, we optimize the Gaussian object. We begin by fusing color point clouds from the keyframes, followed by downsampling with a voxel size of 0.01 m. We then cluster the points with a maximum distance of 0.06m between points to remove outlier points. Subsequently, we uniformly upsample the point cloud until the number of points exceeds 5000.

%Before the joint optimization of 2D Gaussians and poses, the 2D Gaussian parameters are initialized. 
We initialize the Gaussian means with the point cloud positions and random rotations. To simplify training and mitigate floating artifacts caused by oversized splats, Gaussian scales are clipped between 0.005 and 0.01. We use Spherical harmonics to represent the color, beginning at level 0 and incrementing every 200 steps, up to level 2. We initialize the opacity of each Gaussian with 0.1. Pose gradients for each keyframe are initialized with six parameters, (3 for translations and 3 for the rotation in an axis-angle representation). Before optimization, we group the keyframe poses using different anchors based on a default setting of an icosahedron at level 1, yielding a total of 42 anchors. Keyframes with the largest masks in each anchor cluster are selected for joint optimization, which runs for 1000 steps.

After 500 steps, the opacity percentile-based Adaptive Density Control is applied every 100 steps. Gaussians with opacity values in the bottom 5th percentile are removed until the 95th percentile opacity exceeds 0.5. Similarly, every 100 steps, keyframes with reconstruction losses exceeding twice the median absolute deviation (MAD) are removed.

In the training loss, $\lambda_c$ = 0.5, $\lambda_d$ = 0.5, $\lambda_{dd}$ = 0.05, $\lambda_n$ = 0.05. To mitigate depth noise, we apply morphological erosion to the depth using a kernel size of 5. The Adam optimizer is utilized for optimizing both the pose and Gaussian parameters, with a decay rate set to 0.5. The initial learning rate for Gaussians is consistent with the 2DGS~\cite{huang2DGaussianSplatting2024} configuration. After the joint optimization is run for 1000 steps, the Gaussians' attributes are fixed, and only the keyframe poses are further refined for 500 additional steps.

All experiments were performed on a standard desktop equipped with an AMD Ryzen 9 7950X3D 16-core Processor and a single NVIDIA RTX 4090 GPU. Only the temporal efficiency experiments in Sec.~\ref{ssec:temporal-efficiency} used a PC with a different configuration. Our method utilizes two concurrently running threads. The online tracking thread processes frames at approximately 4.1 Hz, while the Gaussian object field thread operates in the background, requiring an average of 0.23 seconds per keyframe.

% \section{Additional Results}
% \begin{itemize}
%     \item HO3D Table and Image with all sequences
%     \item YCBinEOAT Table and Images with all sequences
%     \item BEHAVE Dataset
% \end{itemize}

% \section{Realtime results}

% \textcolor{red}{Real-time experiment figures}

\section{Limitations}
\begin{figure}[h!]
    \centering
    \includegraphics[width=\linewidth]{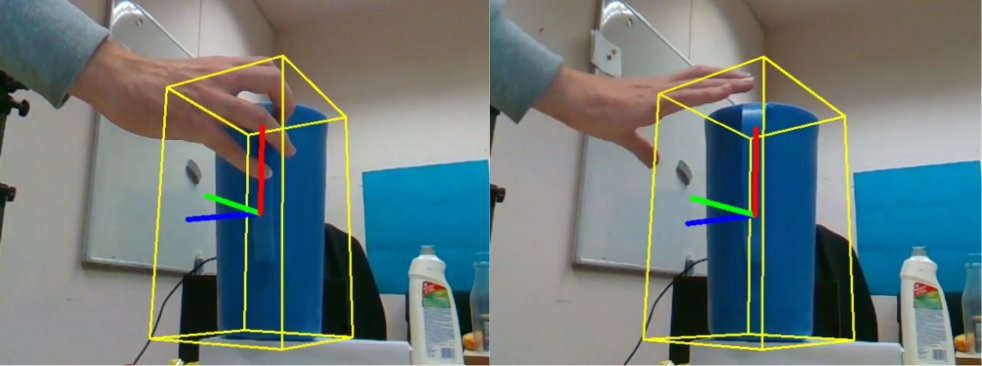}
    \caption{Rotation angle estimation from a side view is often inaccurate for symmetric objects without texture information, as exemplified by the AP10 object from the HO3D dataset.}
    \label{fig:failure_cleaner}
    \vspace{-1em}
\end{figure}

Gaussian rasterization rendering is highly efficient and allows for the rapid correction of minor translation and in-plane rotation errors. However, it is less effective in gradient computation compared to the differentiable ray casting employed by neural radiance fields. This limitation stems from the fact that pose gradients in Gaussian rasterization are approximated using the covariance matrix projected onto the 2D plane. As a result, gradient-based optimization for non-in-plane rotations or substantial pose corrections becomes problematic. For example, our method struggles to resolve rotational errors around the symmetric axis of a water pitcher, as shown in Fig~\ref{fig:failure_cleaner}. 

% % Additionally, for geometrically symmetric objects, such as a spam can with nearly identical front and back textures, distinguishing between the two orientations without prior knowledge is challenging, as illustrated in Fig.
% \section{Realtime Results}
% \TODO{Move this section up to the main paper}

% \begin{figure}[h!]
%     \centering
%     \includegraphics[width=\linewidth]{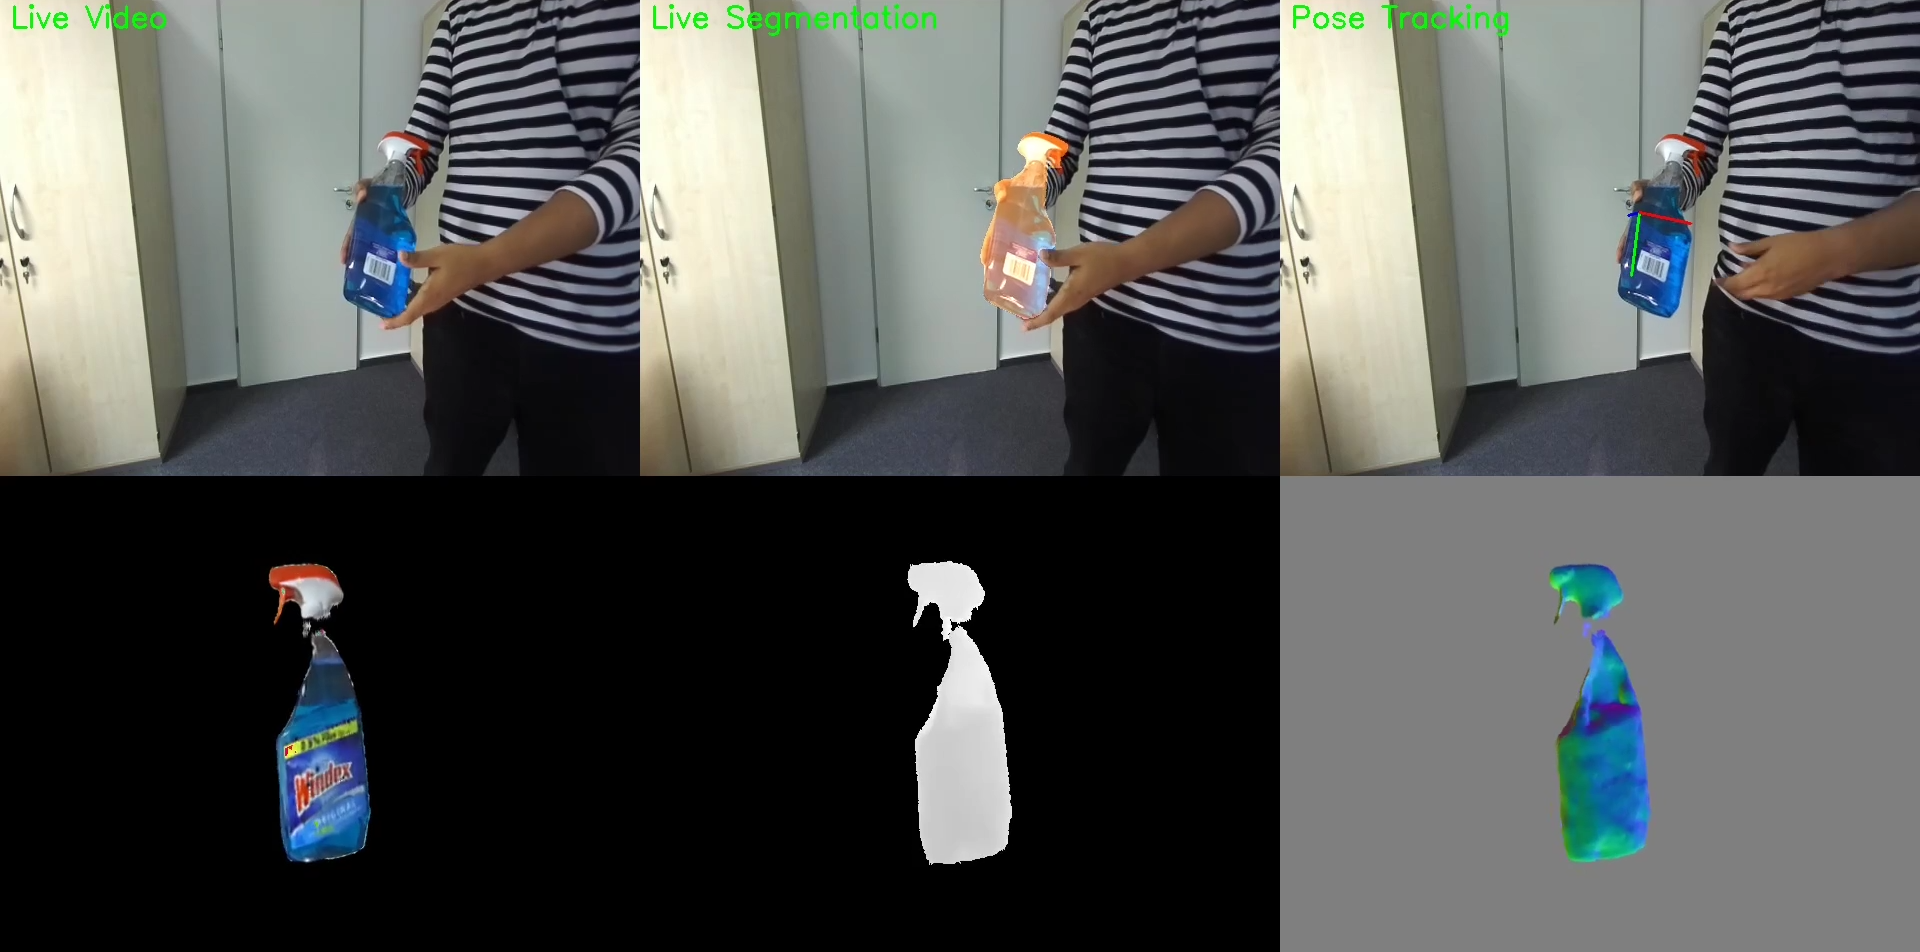}
%     \caption{Example of real-time object tracking. \textbf{Top row:} Live video, object segmentation results, and pose tracking results. \textbf{Bottom row:} Rendered outputs, including color, depth, and surface normals derived from the Gaussian models.}
%     \label{fig:realtime}
%     \vspace{-1em}
% \end{figure}
% We utilized the ZED 2 camera operating in the standard depth sensing mode to maintain a balance between frame rate and accuracy. The camera captures video at a resolution of 1080p with a frame rate of 30 FPS. An initial mask for the target object was manually created through human annotation. The SAM2 system also operates at 28 FPS. Pose tracking, when running in visualization mode, achieves a processing frequency of 3-4 Hz, primarily due to the computational overhead introduced by the GUI and the rendering of Gaussian models in the background. Without the GUI, the system can operate at a slightly higher frequency of 4-5 Hz. The Gaussian model updates approximately every 8 seconds, as illustrated in Fig~\ref{fig:realtime}. For a more comprehensive understanding of the system's performance, we encourage readers to refer to the supplementary video provided.

\section{Additional Ablation}
% Performance was reduced without dynamic keyframe selection (\textit{Ours w/o KF selection}) due to the retention of inaccurate pose estimates during training, which introduces residual errors in the reconstruction loss and hinders pose optimization. Applying the vanilla adaptive density control (\textit{Ours w/o Pruning}), where all Gaussians below a predefined threshold are removed, causes abrupt changes in the number of Gaussians. This results in significant rendering fluctuations, slowing the convergence of training. The pose accuracy and reconstruction quality of 3DGS (\textit{Ours (3DGS)}) are inferior to 2DGS. This can be attributed to the lack of regularization on the normal and depth in 3DGS, causing the Gaussians to deviate from the object surface and consequently degrading the reconstruction quality. We find that our approach with the proposed additions, namely Dynamic Keyframe Selection and the Opacity Percentile-based Adaptive Density Control performs the best among all.

A visual comparison of the different ablations in reconstructing a water pitcher from HO3D can be seen in Fig.~\ref{fig:ablation-reconstruction}. This example is particularly difficult as there are large rotational motions and large occlusions. In this example, we find that neither of the ablations can accurately reconstruct the pitcher, especially the handle. Rather, they end up with two partially reconstructed handles as a result of inaccurate keyframe estimates which cause points to be added from a new keyframe with the handle visible. However, by combining the dynamic keyframe selection and the opacity percentile-based adaptive density control, our final approach reconstructs the handle more accurately.

\begin{figure}[ht!]
    \centering
    \includegraphics[width=\linewidth]{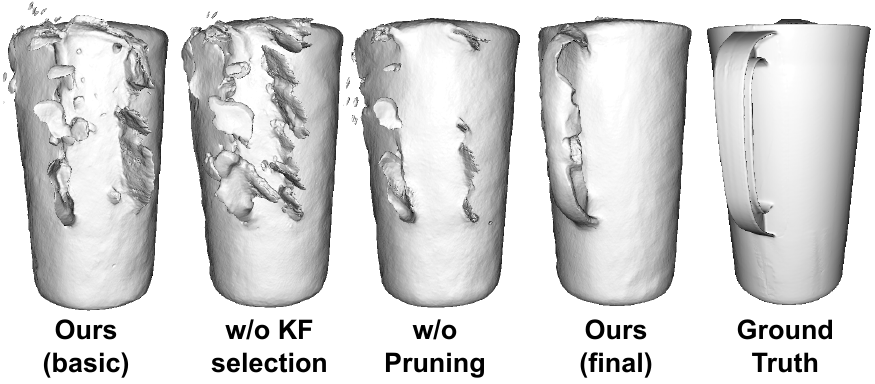}
    \caption{Object reconstruction example using the different ablations over our approach.}
    \label{fig:ablation-reconstruction}
    \vspace{-1em}
\end{figure}

\begin{figure*}
    \centering
    \includegraphics[width=\textwidth]{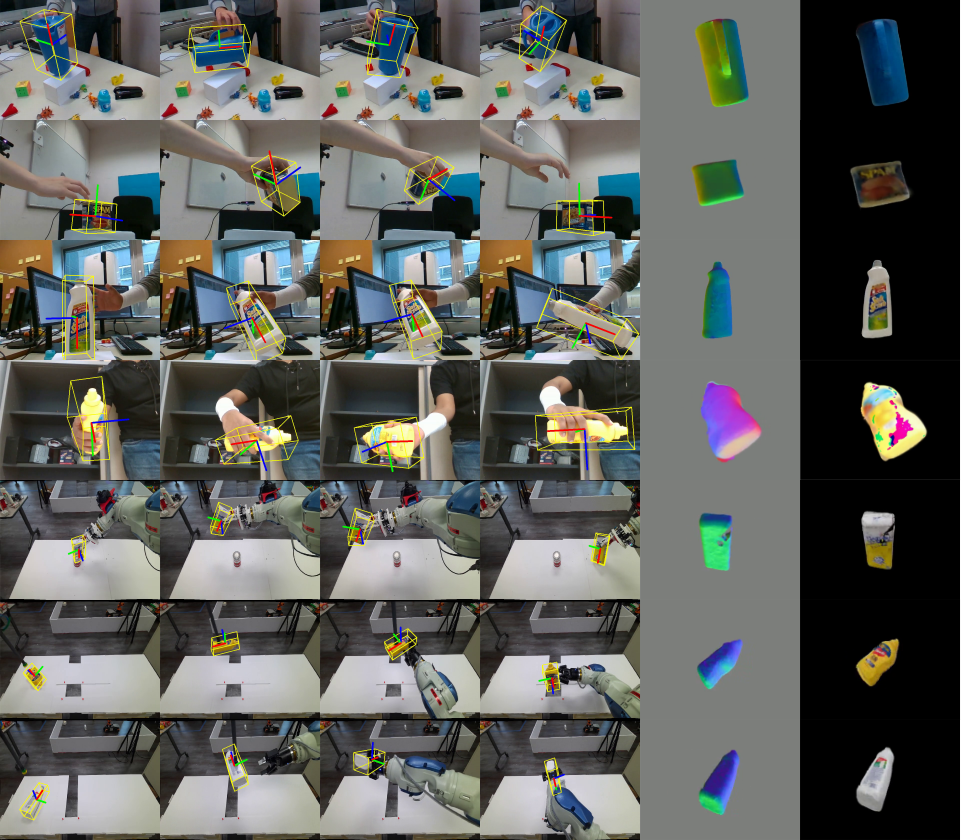}
    \caption{Qualitative results of our method on video sequences from the HO3D and YCBInEOAT datasets}
    \label{fig:ho3_and_ycb_viz}
\end{figure*}

\newpage
\begin{table*}[t]
    \centering
    \caption{Comparison of ADD-S, ADD, and CD metrics, along with the Average Time Per Frame, across different methods on the HO3D dataset. ↑ indicates higher values are better, ↓ indicates lower values are better. The results in the first 2 columns are taken from~\cite{wenBundleSDFNeural6DoF2023}. * highlights the results reproduced using the open-source code from the authors of~\cite{wenBundleSDFNeural6DoF2023}.}
    \label{tab:ho3_table}
    \resizebox{\textwidth}{!}{
% Please add the following required packages to your document preamble:
% \usepackage{multirow}
\begin{tabular}{|c|c|cc|cccc|c|}
\hline
Video & Metric & BundleTrack~\cite{wenBundleTrack6DPose2021} & BundleSDF~\cite{wenBundleSDFNeural6DoF2023} & BundleTrack$^\ast$ & BundleSDF$^\ast$ & BundleSDF-async$^\ast$ & BundleSDF-Lite & Ours \\ \hline
& ADD-S(\%)↑ & 91.68 & 96.1 & 91.24 & \textbf{95.83} & 91.78 & 93.03 & 95.34 \\
 & ADD(\%)↑ & 36.60 & 91 & 47.98 & \textbf{89.66} & 66.38 & 78.66 & 85.88 \\
 & CD(cm)↓ & 1.88 & 0.47 & - & 0.13 & 0.55 & 0.76 & \textbf{0.20} \\
\multirow{-4}{*}{AP10} & ATPF(s)↓ & - & - & 0.27 & 1.55 & 0.26 & 0.39 & \textbf{0.23} \\ \hline
 & ADD-S(\%)↑ & 91.45 & 96.18 & 94.14 & 96.01 & 95.47 & 93.34 & \textbf{96.92} \\
 & ADD(\%)↑ & 41.28 & 91.76 & 84.53 & 90.91 & 89.32 & 81.05 & \textbf{93.78} \\
 & CD(cm)↓ & 129.18 & 0.56 & - & 0.10 & 0.13 & 0.65 & \textbf{0.06} \\
\multirow{-4}{*}{AP11} & ATPF(s)↓ & - & - & 0.28 & 1.46 & 0.26 & 0.38 & \textbf{0.23} \\ \hline
 & ADD-S(\%)↑ & 90.79 & 97.06 & 95.42 & \textbf{96.98} & 96.51 & 93.87 & 96.77 \\
 & ADD(\%)↑ & 50.82 & 94.76 & 88.09 & \textbf{94.53} & 92.32 & 83.34 & 93.35 \\
 & CD(cm)↓ & 2.47 & 0.59 & - & \textbf{0.04} & 0.09 & 0.74 & 0.06 \\
\multirow{-4}{*}{AP12} & ATPF(s)↓ & - & - & 0.29 & 1.40 & 0.28 & 0.41 & \textbf{0.25} \\ \hline
 & ADD-S(\%)↑ & 90.68 & 96.16 & 95.65 & 96.19 & 95.96 & 92.66 & \textbf{96.46} \\
 & ADD(\%)↑ & 49.03 & 92.73 & 89.95 & 92.77 & 92.11 & 80.14 & \textbf{92.90} \\
 & CD(cm)↓ & 2.77 & 0.63 & - & \textbf{0.03} & 0.05 & 0.78 & 0.06 \\
\multirow{-4}{*}{AP13} & ATPF(s)↓ & - & - & 0.28 & 1.40 & 0.29 & 0.41 & \textbf{0.24} \\ \hline
 & ADD-S(\%)↑ & 96.02 & 96.01 & 96.09 & \textbf{97.09} & 96.89 & 96.50 & 95.84 \\
 & ADD(\%)↑ & 90.30 & 91.25 & 91.07 & \textbf{94.65} & 94.11 & 92.23 & 91.56 \\
 & CD(cm)↓ & 72.40 & 1.28 & - & \textbf{0.03} & 0.05 & 0.71 & 0.07 \\
\multirow{-4}{*}{AP14} & ATPF(s)↓ & - & - & 0.29 & 1.46 & 0.29 & 0.41 & \textbf{0.25} \\ \hline
 & ADD-S(\%)↑ & 94.94 & 95.05 & 93.01 & \textbf{95.28} & 93.79 & 93.31 & 94.29 \\
 & ADD(\%)↑ & 87.45 & 88.92 & 75.64 & \textbf{89.48} & 83.75 & 83.78 & 84.55 \\
 & CD(cm)↓ & 0.97 & 0.56 & - & \textbf{0.13} & 0.29 & 0.57 & 0.33 \\
\multirow{-4}{*}{MPM10} & ATPF(s)↓ & - & - & 0.29 & 2.39 & 0.29 & 0.44 & \textbf{0.23} \\ \hline
 & ADD-S(\%)↑ & 89.94 & 96.2 & 96.06 & \textbf{96.19} & 96.53 & 94.75 & 96.09 \\
 & ADD(\%)↑ & 53.20 & 91.51 & 91.07 & 91.51 & 92.33 & 88.44 & \textbf{91.91} \\
 & CD(cm)↓ & 88.97 & 0.49 & - & 0.09 & \textbf{0.09} & 0.53 & 0.12 \\
\multirow{-4}{*}{MPM11} & ATPF(s)↓ & - & - & 0.28 & 2.17 & 0.28 & 0.44 & \textbf{0.27} \\ \hline
 & ADD-S(\%)↑ & 95.66 & 96.98 & 97.88 & 96.17 & 97.18 & 80.20 & \textbf{97.76} \\
 & ADD(\%)↑ & 90.96 & 93.13 & 95.12 & 91.36 & 93.64 & 60.98 & \textbf{95.48} \\
 & CD(cm)↓ & 121.33 & 0.46 & - & 0.08 & \textbf{0.06} & 1.30 & 0.07 \\
\multirow{-4}{*}{MPM12} & ATPF(s)↓ & - & - & 0.34 & 1.93 & 0.33 & 0.49 & \textbf{0.22} \\ \hline
 & ADD-S(\%)↑ & 89.42 & 95.8 & 85.37 & 74.70 & 65.79 & 54.19 & \textbf{88.00} \\
 & ADD(\%)↑ & 38.78 & 90.62 & 32.03 & 51.91 & 26.39 & 27.51 & \textbf{32.50} \\
 & CD(cm)↓ & 81.39 & 0.57 & - & \textbf{0.90} & 1.67 & 0.92 & 2.06 \\
\multirow{-4}{*}{MPM13} & ATPF(s)↓ & - & - & 0.27 & 1.83 & 0.27 & 0.36 & \textbf{0.25} \\ \hline
 & ADD-S(\%)↑ & 95.49 & 97.33 & 95.49 & \textbf{97.19} & 95.44 & 96.63 & 95.55 \\
 & ADD(\%)↑ & 90.16 & 94.52 & 88.02 & \textbf{94.18} & 87.75 & 92.43 & 88.88 \\
 & CD(cm)↓ & 94.99 & 0.47 & - & \textbf{0.07} & 0.30 & 0.50 & 0.24 \\
\multirow{-4}{*}{MPM14} & ATPF(s)↓ & - & - & \textbf{0.30} & 2.41 & 0.30 & 0.44 & 0.59 \\ \hline
 & ADD-S(\%)↑ & 94.44 & 97.27 & 94.54 & \textbf{97.07} & 94.40 & 95.17 & 94.55 \\
 & ADD(\%)↑ & 84.64 & 94.39 & 78.34 & \textbf{93.82} & 79.13 & 86.53 & 78.23 \\
 & CD(cm)↓ & 75.83 & 0.46 & - & \textbf{0.12} & 0.58 & 0.60 & 0.63 \\
\multirow{-4}{*}{SB11} & ATPF(s)↓ & - & - & 0.23 & 2.18 & 0.23 & 0.37 & 0.59 \\ \hline
 & ADD-S(\%)↑ & 95.66 & 97.67 & 97.28 & \textbf{97.71} & 97.20 & 96.99 & 97.08 \\
 & ADD(\%)↑ & 85.47 & 95.24 & 92.68 & \textbf{95.31} & 92.90 & 92.09 & 92.30 \\
 & CD(cm)↓ & 2.49 & 0.47 & - & \textbf{0.08} & 0.16 & 0.75 & 0.17 \\
\multirow{-4}{*}{SB13} & ATPF(s)↓ & - & - & 0.25 & 1.82 & 0.25 & 0.39 & \textbf{0.22} \\ \hline
 & ADD-S(\%)↑ & 84.94 & 96.9 & 89.36 & \textbf{96.87} & 89.39 & 87.44 & 91.31 \\
 & ADD(\%)↑ & 59.41 & 94.24 & 56.13 & \textbf{94.19} & 58.27 & 57.03 & 75.05 \\
 & CD(cm)↓ & 2.04 & 0.44 & - & \textbf{0.08} & 1.43 & 0.91 & 0.77 \\
\multirow{-4}{*}{SM1} & ATPF(s)↓ & - & - & 0.33 & 5.25 & 0.34 & 0.74 & \textbf{0.27} \\ \hline
 & ADD-S(\%)↑ & 92.39 & 96.52 & 93.96 & 94.87 & 92.80 & 89.85 & \textbf{95.07} \\
 & ADD(\%)↑ & 66.01 & 92.62 & 77.75 & \textbf{89.56} & 80.65 & 77.25 & 84.34 \\
 & CD(cm)↓ & 52.05 & 0.57 & - & \textbf{0.15} & 0.42 & 0.75 & 0.41 \\
\multirow{-4}{*}{Mean} & ATPF(s)↓ & - & - & 0.29 & 2.10 & 0.28 & 0.44 & \textbf{0.24} \\ \hline
\end{tabular}
    }
\end{table*}

% Please add the following required packages to your document preamble:
% \usepackage{multirow}
% \usepackage[table,xcdraw]{xcolor}
% Beamer presentation requires \usepackage{colortbl} instead of \usepackage[table,xcdraw]{xcolor}
\newpage
\begin{table*}[t]
    \centering
    \caption{Comparison of ADD-S, ADD, and CD metrics, along with the Average Time Per Frame, across different methods on the YCBInEOAT dataset. ↑ indicates higher values are better, ↓ indicates lower values are better. The results in the first 2 columns are taken from~\cite{wenBundleSDFNeural6DoF2023}. * highlights the results reproduced using the open-source code from the authors of~\cite{wenBundleSDFNeural6DoF2023}.}
    \label{tab:ycb_table}
    \resizebox{\textwidth}{!}{
% Please add the following required packages to your document preamble:
% \usepackage{multirow}
\begin{tabular}{|c|c|cc|cccc|c|}
\hline
Object & Metric & BundleTrack~\cite{wenBundleTrack6DPose2021} & BundleSDF~\cite{wenBundleSDFNeural6DoF2023} & BundleTrack$^\ast$ & BundleSDF$^\ast$ & BundleSDF-async$^\ast$ & BundleSDF-Lite & Ours \\ \hline
 & ADD-S(\%)↑ & 90.2 & 90.63 & 89.41 & 90.23 & 91.78 & 90.52 & \textbf{95.33} \\
 & ADD(\%)↑ & 85.08 & 85.37 & 63.24 & 80.29 & 66.38 & 81.99 & \textbf{91.3} \\
 & CD(cm)↓ & 1.36 & 0.76 & - & 0.53 & 0.55 & 0.21 & \textbf{0.1} \\
\multirow{-4}{*}{cracker\_box} & ATPF(s)↓ & - & \textbf{-} & 0.20 & 0.59 & 0.20 & 0.21 & \textbf{0.18} \\ \hline
 & ADD-S(\%)↑ & 95.22 & 94.28 & 82.45 & 93.48 & 95.47 & 92.18 & \textbf{93.81} \\
 & ADD(\%)↑ & 89.34 & 87.46 & 61.83 & 85.48 & 89.32 & 82.56 & \textbf{85.78} \\
 & CD(cm)↓ & 1.31 & 0.53 & - & 0.44 & \textbf{0.13} & 0.16 & 0.25 \\
\multirow{-4}{*}{bleach\_cleanser} & ATPF(s)↓ & - & \textbf{-} & \textbf{0.21} & 1.01 & 0.22 & 0.23 & \textbf{0.21} \\ \hline
 & ADD-S(\%)↑ & 90.68 & 93.81 & 81.42 & \textbf{96.58} & 96.51 & 89.48 & 96.21 \\
 & ADD(\%)↑ & 85.49 & 88.62 & 51.91 & 92.08 & 92.32 & 82.33 & \textbf{92.34} \\
 & CD(cm)↓ & 2.25 & 0.46 & - & 0.23 & 0.09 & 0.22 & \textbf{0.07} \\
\multirow{-4}{*}{sugar\_box} & ATPF(s)↓ & - & \textbf{-} & \textbf{0.20} & 0.70 & 0.22 & 0.26 & 0.21 \\ \hline
 & ADD-S(\%)↑ & 95.24 & 95.24 & 71.61 & 79.19 & \textbf{95.96} & 94.84 & 94.26 \\
 & ADD(\%)↑ & 85.78 & 83.1 & 41.36 & 57.3 & \textbf{92.11} & 82.45 & 86.14 \\
 & CD(cm)↓ & 7.36 & 3.57 & - & 1.16 & \textbf{0.05} & 0.35 & 0.28 \\
\multirow{-4}{*}{tomato\_soup\_can} & ATPF(s)↓ & - & \textbf{-} & \textbf{0.20} & 1.07 & 0.20 & 0.25 & 0.23 \\ \hline
 & ADD-S(\%)↑ & 95.84 & 95.75 & 88.53 & 95.85 & 96.89 & 95.07 & \textbf{95.94} \\
 & ADD(\%)↑ & 92.15 & 89.87 & 71.92 & 90.15 & \textbf{94.11} & 86.95 & 92.22 \\
 & CD(cm)↓ & 1.76 & 0.45 & - & 0.31 & \textbf{0.05} & 0.18 & 0.12 \\
\multirow{-4}{*}{mustard\_bottle} & ATPF(s)↓ & - & \textbf{-} & \textbf{0.21} & 0.74 & 0.22 & 0.26 & 0.25 \\ \hline
 & ADD-S(\%)↑ & 93.01 & 92.77 & 81.17 & 92.82 & 92.79 & 92.66 & \textbf{93.79} \\
 & ADD(\%)↑ & 87.26 & 86.95 & 57.91 & 84.28 & 83.75 & 83.41 & \textbf{87.83} \\
 & CD(cm)↓ & 2.81 & 1.16 & - & 0.53 & 0.29 & 0.25 & \textbf{0.15} \\
\multirow{-4}{*}{Mean} & ATPF(s)↓ & - & \textbf{-} & \textbf{0.21} & 0.82 & \textbf{0.21} & 0.24 & 0.22 \\ \hline
\end{tabular}
}
\end{table*}
